# Supplementary material for: Unveiling the Risks of NFT Promotion Scams
Source: arXiv:2301.09806 source file (2023-09-11)
Supplement: Supplementary file 1 [file appendix.tex]

\section{Appendix}

% \begin{table}[]
% \caption{Descriptive statistics of accounts which \textit{promoted} NFT collections (n=439)}
% \label{table:desc-promoters}
% \resizebox{0.95\columnwidth}{!}{
% \begin{tabular}{l|llll}
% \hline
% \hline
% Feature & Min & Max & Mean & Median \\ \hline
% Followers & 40,041 & 2,510,942 & 184152.6 & 104,743 \\ 
% Friends & 0 & 136,762 & 2932.1 & 318 \\ 
% Tweets & 196 & 325,776 & 15427.7 & 4767 \\ 
% Listed count & 0 & 4,460 & 469.8 & 98.5 \\ 
% Age (in days) & 102 & 5529 & 867 & 379 \\ \hline \hline
% \end{tabular}}
% \end{table}
